# Supplementary material for: Regret Minimization in Stackelberg Games with Side Information
Source: arXiv:2402.08576 source file (2024-10-12)
Supplement: Supplementary file 1 [file ftpl.tex]

\section{Appendix for~\Cref{sec:ftpl}: New Results for FTPL with Bandit Feedback}
\textbf{Full-feedback algorithm} 

\noindent For each time $t \in [T]$:
\begin{enumerate}
    \item Draw a random sequence of follower types $\{g^{(1)}, \ldots, g^{(k)}\}$ independently via geometric sample perturbations
    \item Let $f_1, \ldots, f_{t-1}$ be the sequence of follower types seen so far
    \item Play mixed strategy
    \begin{equation*}
        \vx_t = \arg\max_{\vx \in \cX} \left( \sum_s u(\vx, b_{g^{(s)}}(\vx)) + \sum_{s=1}^{t-1} u(\vx, b_{f_s}(\vx)) \right)
    \end{equation*}
\end{enumerate}

\noindent \textbf{Bandit feedback idea}

\noindent For each time $t \in [T]$:
\begin{enumerate}
    \item Draw a random sequence of follower types $\{g^{(1)}, \ldots, g^{(k)}\}$ independently via geometric sample perturbations
    %
    %\item Compute an unbiased estimate of the proportion of $\{\alpha^{(1)}, \ldots, \alpha^{(K)}\}$ seen so far as $\widehat{\mathbb{P}}_t(\alpha^{(i)})$ for $i \in [K]$
    %
    \item Compute an unbiased estimate of $\bP(b_{f_t}(\vx) = a_f)$ as $\widehat{\bP}(b_{f_t}(\vx) = a_f)$ for all $x \in \cE$, $a_f \in \cA_f$
    \begin{itemize}
        \item $\bP(b_{f,t}(\vx) = a)$ should be read as ``the probability that follower $f_t$ takes action $a \in \cA_f$, given that the leader plays a mixed strategy $\vx$
        \item $\sigma(\vx)$ is the best-response region which mixed strategy $\vx$ belongs to, i.e. $\vx \in \sigma$
    \end{itemize}
    %
    \iffalse
    \item Play mixed strategy
    %
    \begin{equation*}
        \vx_t = \arg\max_{\vx \in \cX} \left( \sum_s U(\vx, g^{(s)}) + (t-1) \sum_{i=1}^{K}  \widehat{\mathbb{P}}_t(\alpha^{(i)}) \cdot U(\vx, \alpha^{(i)}) \right)
    \end{equation*}
    \fi 
    %
    \item Play mixed strategy
    \begin{equation*}
    \begin{aligned}
        \vx_t &= \arg\max_{\vx \in \cX} \left( \sum_s u(\vx, b_{g^{(s)}}(\vx)) + \sum_{\tau=1}^{t-1} \sum_{a_f \in \cA_f}  \widehat{\mathbb{P}}(b_{f_\tau}(\vx) = a_f) \cdot u(\vx, a_f) \right)\\
        &= \arg\max_{\vx \in \cX} \left( \sum_s \sum_{a_f \in \cA_f} \bP(b_{g^{(s)}}(\vx) = a_f) \cdot u(\vx, a_f) + \sum_{\tau=1}^{t-1} \sum_{a_f \in \cA_f}  \widehat{\mathbb{P}}(b_{f_\tau}(\vx) = a_f) \cdot u(\vx, a_f) \right)\\
    \end{aligned}
    \end{equation*}
    \begin{itemize}
        \item Observe that if $\widehat{\mathbb{P}}(b_{f_\tau}(\vx) = a_f) = \mathbb{P}(b_{f_\tau}(\vx) = a_f)$, $\forall \tau$, then we recover the full-feedback version of FTPL
    \end{itemize}
\end{enumerate}
\paragraph{Notation}
\begin{itemize}
    %
    %\item Let $\vf_t := [\mathbbm{1}\{f_t = \alpha^{(1)}\} \; \dots \; \mathbbm{1}\{f_t = \alpha^{(K)}\} \}]^\top$
    %
    \item Let $\vp_{\vx, f_t} := [\mathbbm{1}\{b_{f_t}(\vx) = a\}]_{a \in \cA_f} = [\bP(b_{f_t}(\vx) = a)]_{a \in \cA_f}$, $\vp_{f_t} = \{\vp_{\vx, f_t}\}_{\vx \in \cE}$. 
    \begin{itemize}
        \item Observe that $\vp_{\vx, f_t} = \vp_{\vx', f_t}$ for all $\vx, \vx' \in \sigma$
    \end{itemize}
    %
    %\item Let $\widehat{\vf}_t := [\widehat{\bP}(f_t = \alpha^{(1)}) \; \dots \; \widehat{\bP}(f_t = \alpha^{(K)})]^\top$
    %
    \item Let $\widehat{\vp}_{\vx, f_t} := [\widehat{\bP}(b_{f_t}(\vx) = a)]_{a \in \cA_f}$, $\widehat{\vp}_t = \{\widehat{\vp}_{\vx, f_t}\}_{\vx \in \cE}$
    %
    %\item Assume $\E[\widehat{\vf}_t] = \vf_t$ and that $\widehat{\vf}_t$ is bounded
    %
    \item Assume $\E[\widehat{\vp}_{\vx, f_t}] = \vp_{\vx, f_t}$ and that $\widehat{\vp}_{\vx, f_t} \in [-\kappa, \kappa]^{A_f}$
    %
    %\item $u(\vx, \widehat{f}_t) = \sum_{i=1}^K u(\vx, \alpha^{(i)}) \cdot \widehat{\bP}(f_t = \alpha^{(i)}) = \langle \mathbf{u}(\vx, \cdot), \widehat{\vf}_t \rangle$
    %
    \item $u(\vx, \vp_{f_t}) = \sum_{a_f \in \cA_f} u(\vx, a_f) \cdot \bP(b_{f_t}(\vx) = a_f) = \langle \mathbf{u}(\vx, \cdot), \vp_{\vx, f_t} \rangle$
    \item $u(\vx, \widehat{\vp}_{f_t}) = \sum_{a_f \in \cA_f} u(\vx, a_f) \cdot \widehat{\bP}(b_{f_t}(\vx) = a_f) = \langle \mathbf{u}(\vx, \cdot), \widehat{\vp}_{\vx, f_t} \rangle$
    %
    %\item $U(\vx, f_{1:\tau}) := \sum_{t=1}^\tau u(\vx, f_t)$
    %
    \item $U(\vx, \vp_{f_{1:\tau}}) := \sum_{t=1}^\tau u(\vx, \vp_{f_t})$
    %
    %\item $U(\vx, \widehat{f}_{1:\tau}) := \sum_{t=1}^\tau u(\vx, \widehat{f}_t)$
    %
    \item $U(\vx, \widehat{\vp}_{f_{1:\tau}}) := \sum_{t=1}^\tau u(\vx, \widehat{\vp}_{f_t})$
    %
    %\item $M(f_{1:\tau}) := \arg\max_{\vx \in \cX} U(\vx, f_{1:\tau})$
    %
    \item $M(\vp_{f_{1:\tau}}) := \arg\max_{\vx \in \cX} U(\vx, \vp_{f_{1:\tau}})$
    %
    %\item $M(\widehat{f}_{1:\tau}) := \arg\max_{\vx \in \cX} U(\vx, \widehat{f}_{1:\tau})$
    %
    \item $M(\widehat{\vp}_{f_{1:\tau}}) := \arg\max_{\vx \in \cX} U(\vx, \widehat{\vp}_{f_{1:\tau}})$
\end{itemize}
%
% \begin{lemma}[Be the Estimated Leader]\label{lem:btel}
%     \begin{equation*}
%         \sum_{t=1}^T u(M(\widehat{f}_{1:t}), \widehat{f}_t) \geq \max_{\vx \in \cX} U(\vx, \widehat{f}_{1:T})
%     \end{equation*}
% \end{lemma}
% %
% \begin{proof}
%     Inductive hypothesis: $\sum_{t=1}^\tau u(M(\widehat{f}_{1:t}), \widehat{f}_t) \geq \sum_{t=1}^\tau u(M(\widehat{f}_{1:\tau}), \widehat{f}_t)$
%     %
%     \begin{equation*}
%     \begin{aligned}
%         \sum_{t=1}^{\tau+1} u(M(\widehat{f}_{1:t}), \widehat{f}_t) &= \sum_{t=1}^\tau u(M(\widehat{f}_{1:t}), \widehat{f}_t) + u(M(\widehat{f}_{1:\tau+1}), \widehat{f}_{\tau+1})\\
%         %
%         &\geq \sum_{t=1}^\tau u(M(\widehat{f}_{1:\tau}), \widehat{f}_t) + u(M(\widehat{f}_{1:\tau+1}), \widehat{f}_{\tau+1})\\
%         %
%         &\geq \sum_{t=1}^\tau u(M(\widehat{f}_{1:\tau+1}), \widehat{f}_t) + u(M(\widehat{f}_{1:\tau+1}), \widehat{f}_{\tau+1})\\
%         &= \sum_{t=1}^{\tau+1} u(M(\widehat{f}_{1:\tau+1}), \widehat{f}_t)
%     \end{aligned}
%     \end{equation*}
% \end{proof}
%
\begin{lemma}[Be the Estimated Leader]\label{lem:btel}
    \begin{equation*}
        \sum_{t=1}^T u(M(\widehat{\vp}_{f_{1:t}}), \widehat{\vp}_{f_t}) \geq \max_{\vx \in \cE} U(\vx, \widehat{\vp}_{f_{1:T}})
    \end{equation*}
\end{lemma}
\begin{proof}
    Inductive hypothesis: $\sum_{t=1}^\tau u(M(\widehat{\vp}_{f_{1:t}}), \widehat{\vp}_{f_t}) \geq \sum_{t=1}^\tau u(M(\widehat{\vp}_{f_{1:\tau}}), \widehat{\vp}_{f_t})$
    \begin{equation*}
    \begin{aligned}
        \sum_{t=1}^{\tau+1} u(M(\widehat{\vp}_{f_{1:t}}), \widehat{\vp}_{f_t}) &= \sum_{t=1}^\tau u(M(\widehat{\vp}_{f_{1:t}}), \widehat{\vp}_{f_t}) + u(M(\widehat{\vp}_{f_{1:\tau+1}}), \widehat{\vp}_{f_{\tau+1}})\\
        &\geq \sum_{t=1}^\tau u(M(\widehat{\vp}_{f_{1:\tau}}), \widehat{\vp}_{f_t}) + u(M(\widehat{\vp}_{f_{1:\tau+1}}), \widehat{\vp}_{f_{\tau+1}})\\
        &\geq \sum_{t=1}^\tau u(M(\widehat{\vp}_{f_{1:\tau+1}}), \widehat{\vp}_{f_t}) + u(M(\widehat{\vp}_{f_{1:\tau+1}}), \widehat{\vp}_{f_{\tau+1}})\\
        &= \sum_{t=1}^{\tau+1} u(M(\widehat{\vp}_{f_{1:\tau+1}}), \widehat{\vp}_{f_t})
    \end{aligned}
    \end{equation*}
\end{proof}
%
% \begin{lemma}\label{lem:martingale}
%     %
%     Suppose that $\E[\widehat{f}_t] = f_t$ and $\widehat{f}_t \in [-\kappa, \kappa]$ for $t \in [T]$, where $\kappa \geq 1$. 
%     %
%     Then $\sum_{t=1}^\tau u(M(\{g\} \cup \widehat{f}_{1:\tau-1}), \widehat{f}_{\tau}) - u(M(\{g\} \cup \widehat{f}_{1:\tau-1}), f_{\tau})$ is a martingale with bounded increments of size at most $2K\kappa$. 
% \end{lemma}
%
% \begin{proof}
%     \begin{equation*}
%     \begin{aligned}
%         &\E[\sum_{t=1}^\tau u(M(\{g\} \cup \widehat{f}_{1:\tau-1}), \widehat{f}_{\tau}) - u(M(\{g\} \cup \widehat{f}_{1:\tau-1}), f_{\tau}) | \mathcal{F}_{\tau-1}]\\
%         %
%         = &\sum_{t=1}^\tau \langle u(M(\{g\} \cup \widehat{f}_{1:\tau-1}), \cdot), \E[\widehat{f}_{\tau} - f_{\tau}]\rangle = 0
%     \end{aligned}
%     \end{equation*}
%     $\widehat{f}_{\tau} \in [-\kappa, \kappa]^K$, $f_{\tau} \in [0, 1]^K$, and $u(\vx, \cdot) \in [-1, 1]^K$, and so each increment is at most $2K\kappa$. 
% \end{proof}
%
\begin{lemma}\label{lem:martingale}
    Suppose that $\E[\widehat{\vp}_{f_t}] = \vp_{f_t}$ and $\widehat{\vp}_{f_t} \in [-\kappa, \kappa]^{|\Sigma| \cdot A_f}$ for $t \in [T]$, where $\kappa \geq 1$. 
    Then $\sum_{t=1}^\tau u(M(\{\vp_g\} \cup \widehat{\vp}_{f_{1:\tau-1}}), \widehat{\vp}_{f_{\tau}}) - u(M(\{\vp_g\} \cup \widehat{\vp}_{f_{1:\tau-1}}), \vp_{f_{\tau}})$ is a martingale with bounded increments of size at most $2A_f \kappa$. 
\end{lemma}
\begin{proof}
    \begin{equation*}
    \begin{aligned}
        &\E[\sum_{t=1}^\tau u(M(\{\vp_g\} \cup \widehat{\vp}_{1:\tau-1}), \widehat{\vp}_{\tau}) - u(M(\{\vp_g\} \cup \widehat{\vp}_{1:\tau-1}), \vp_{\tau}) | \mathcal{F}_{\tau-1}]\\
        = &\sum_{t=1}^\tau \langle u(M(\{\vp_g\} \cup \widehat{\vp}_{1:\tau-1}), \cdot), \E[\widehat{\vp}_{\sigma(M(\{\vp_g\} \cup \widehat{\vp}_{1:\tau-1})), \tau} - \vp_{\sigma(M(\{\vp_g\} \cup \widehat{\vp}_{1:\tau-1})), \tau} | \cF_{\tau-1}]\rangle = 0
    \end{aligned}
    \end{equation*}
    $\widehat{\vp}_{\sigma(M(\{\vp_g\} \cup \widehat{\vp}_{1:\tau-1})), \tau} \in [-\kappa, \kappa]^{A_f}$, $\vp_{\sigma(M(\{\vp_g\} \cup \widehat{\vp}_{1:\tau-1})), \tau} \in [0, 1]^{A_f}$, and $u(\vx, \cdot) \in [-1, 1]^{A_f}$, and so each increment is at most $2A_f\kappa$. 
\end{proof}
\begin{theorem}
    Suppose the leader plays FTPL with bandit feedback and geometric sample perturbations with parameter $p = \sqrt{\frac{K}{2T}}$. Then the expected regret is bounded as 
    \begin{equation*}
        \E[R(T)] \leq 4 \sqrt{KT} + 4\sqrt{A_f\kappa T \log T}.
    \end{equation*}
    If $\kappa = K$, then 
    \begin{equation*}
        \E[R(T)] \leq 8\sqrt{A_f K T \log T}.
    \end{equation*}
\end{theorem}
\begin{proof}
    \begin{equation*}
    \begin{aligned}
        \E[R(T)] &:= \E \left[ \max_{\vx \in \cX} \sum_{t=1}^T u(\vx, \vp_{f_t}) - u(M(\{\vp_g\} \cup \widehat{\vp}_{f_{1:t-1}}), \vp_{f_t}) \right]\\
        &= \E \left[ \max_{\vx \in \cX} \sum_{t=1}^T u(\vx, \vp_{f_t}) - u(M(\{\vp_g\} \cup \widehat{\vp}_{f_{1:t-1}}), \widehat{\vp}_{f_t}) + u(M(\{\vp_g\} \cup \widehat{\vp}_{f_{1:t-1}}), \widehat{\vp}_{f_t}) - u(M(\{\vp_g\} \cup \vp_{f_{1:t-1}}), \vp_{f_t}) \right]\\        
        &\leq \E \left[ \max_{\vx \in \cX} \sum_{t=1}^T u(\vx, \vp_{f_t}) - u(M(\{\vp_g\} \cup \widehat{\vp}_{f_{1:t-1}}), \widehat{\vp}_{f_t}) \right] + 4\sqrt{A_f \kappa T\log T}\\
        &= \E \left[ \max_{\vx \in \cX} \sum_{t=1}^T u(\vx, \vp_{f_t}) - u(M(\{\vp_g\} \cup \widehat{\vp}_{f_{1:t}}), \widehat{\vp}_{f_t}) + u(M(\{\vp_g\} \cup \widehat{\vp}_{f_{1:t}}), \widehat{\vp}_{f_t}) - u(M(\{\vp_g\} \cup \widehat{\vp}_{f_{1:t-1}}), \widehat{\vp}_{f_t}) \right]\\ &+ 4\sqrt{A_f \kappa T\log T}\\
        &\leq \max_{\vx \in \cX} \sum_{t=1}^T u(\vx, \vp_{f_t}) - \E \left[ \sum_{t=1}^T u(M(\{\vp_g\} \cup \widehat{\vp}_{f_{1:t}}), \widehat{\vp}_{f_t}) \right] + \sum_{t=1}^T \E[g(t)] + 4\sqrt{A_f \kappa T\log T}\\
        &= \max_{\vx \in \cX} \sum_{t=1}^T \E[ u(\vx, \widehat{\vp}_{f_t})] - \E \left[ \sum_{t=1}^T u(M(\{\vp_g\} \cup \widehat{\vp}_{f_{1:t}}), \widehat{\vp}_{f_t}) \right] + \sum_{t=1}^T \E[g(t)] + 4\sqrt{A_f \kappa T\log T}\\
        &\leq \E \left[ \max_{\vx \in \cX} \sum_{t=1}^T u(\vx, \widehat{\vp}_{f_t}) \right] - \E \left[ \sum_{t=1}^T u(M(\{\vp_g\} \cup \widehat{\vp}_{f_{1:t}}), \widehat{\vp}_{f_t}) \right] + \sum_{t=1}^T \E[g(t)] + 4\sqrt{A_f \kappa T\log T}\\
        &= \E \left[ \max_{\vx \in \cX} \sum_{t=1}^T u(\vx, \widehat{\vp}_{f_t}) - u(M(\{\vp_g\} \cup \widehat{\vp}_{f_{1:t}}), \widehat{\vp}_{f_t}) \right] + \sum_{t=1}^T \E[g(t)] + 4\sqrt{A_f \kappa T\log T}\\
        &\leq \frac{K}{p} +  4\sqrt{A_f \kappa T\log T} + \sum_{t=1}^T \E[g(t)]\\
        %
        %&\leq \frac{K}{p} + 2Tp + 4\sqrt{A_f \kappa T\log T}\\
        %
        %&\leq 4\sqrt{KT} + 4\sqrt{A_f \kappa T\log T}
    \end{aligned}
    \end{equation*}
    where the first inequality follows from~\Cref{lem:martingale} and the Azuma-Hoeffding inequality, 
    the second inequality follows from the definition $u(M(\{\vp_g\} \cup \widehat{\vp}_{f_{1:t}}), \widehat{\vp}_{f_t}) - u(M(\{\vp_g\} \cup \widehat{\vp}_{f_{1:t-1}}), \widehat{\vp}_{f_t}) \leq g(t)$, 
    the third inequality follows from Jensen's inequality.
    the fourth inequality follows from applying~\Cref{lem:btel} (be-the-estimated-leader) to the sequence $\{\vp_g\} \cup \widehat{\vp}_{1:T}$ and the proof of Theorem 25 in~\citet{daskalakis2016learning}, 
    %
    %the fifth inequality follows from Lemma 28 in~\citet{daskalakis2016learning}, 
    %
    %and the final result follows from our choice of $p$. 
    %
    %To see why the fifth inequality follows from Lemma 28 in~\citet{daskalakis2016learning}, observe that the logic in Lemma 28 only depends on properties of the sampling procedure holds for any sequence of follower types $\{f_t\}_{t \in [T]}$. 
    %
    %Therefore, 
\end{proof}

\paragraph{End-to-end algorithm}
\begin{algorithm}[h]
        \SetAlgoNoLine
        \KwIn{Spanning mixed strategies $\vx^{(1)}, \ldots, \vx^{(K)}$}
        \For{$z = 1, \ldots, Z$}
        {
            Pick a random permutation of $K$, along with $K$ uniformly random time-steps $\cK$ in block $z$ and assign them to the exploration phase.\\
            \For{$t=1, \ldots, B$}{
                \uIf{$t \in \cK$}{
                    Play explore strategy $\vx_t = \vx^{(k(t))}$, observe follower action $a_{f,t}$
                }\Else{
                    Play exploit strategy $\vx_{t} = \vx_{z}$
                }
            }
            $\{\widehat{\bP}_z(\alpha)\}_{\alpha \in K} = \texttt{create\_unbiased\_estimate}(\{(\vx_t, a_{f,t})\}_{t \in \cK})$\\
            Set exploit strategy $\vx_{z+1} = \texttt{FTPL}(\{\widehat{\bP}_{z}(\alpha)\}_{\alpha \in K})$
        }
        \caption{Learning in Stackelberg games with bandit feedback.}
        \label{alg:main}
\end{algorithm}
\begin{theorem}\label{thm:ftpl-bandit}
    If $Z = \frac{4T^{2/3} \kappa^{1/3}}{K^{1/3}}$ then \Cref{alg:main} obtains expected regret 
    \begin{equation*}
        E[R(T)] = 8K^{2/3} A_f^{1/3} T^{2/3} \log^{1/3}(T)
    \end{equation*}
    against an oblivious adversary. 
\end{theorem}
\begin{proof}
    \begin{equation*}
    \begin{aligned}
        \E[R(T)] &:= \mathbb{E}[\sum_{t=1}^T u(\vx^*, f_t) - u(\vx_t, f_t)]\\
        &= \E[\sum_{\tau=1}^Z \sum_{t \in B_\tau} u(\vx^*, f_t) - u(\vx_t, f_t)]\\
        &\leq ZK + \E[\sum_{\tau=1}^Z \sum_{t \in B_\tau} u(\vx^*, f_t) - u(\vx_{\tau}, f_t)]\\
        &= ZK + \frac{T}{Z} \cdot \E[\sum_{\tau=1}^Z u(\vx^*, \vf_\tau) - u(\vx_{\tau}, f_{\tau})]\\
        &\leq ZK + \frac{T}{Z} \cdot 8 \sqrt{Z A_f \kappa \log T}\\
        &= 8T^{2/3} \kappa^{1/3} K^{1/3} A_f^{1/3} \log^{1/3}(T)\\
        &= 8K^{2/3} A_f^{1/3} T^{2/3} \log^{1/3}(T)
    \end{aligned}
    \end{equation*}
    where the third line follows from the fact that utilities are bounded between $0$ and $1$, the fourth line follows from the fact that the leader's utility is linear in the follower's type, the fifth line follows from~\Cref{thm:ftpl-bandit} and the fact that $Z \leq T$, the sixth line follows from setting $Z = \frac{4T^{2/3} A_f^{1/3} \kappa^{1/3} \log^{1/3}(T)}{K^{2/3}}$, and the last line follows from the observation that $\kappa = K$. 
\end{proof}
\begin{remark}
    One can get best-of-both-worlds performance when the time horizon is unknown by first playing~\Cref{alg:main} with a doubling trick until a ``cutoff time'', then switching to the algorithm of~\citet{balcan2015commitment} with a doubling trick for the remainder of the time. \khcomment{(Can formalize later)}
\end{remark}
FTPL:
\begin{equation*}
\begin{aligned}
    \vx_{\tau} &= \arg\max_{\vx \in \cE} \sum_{s} u(\vx, b_{f_s}(\vx)) + \sum_{s=1}^{t-1} \widehat{u}_t(\vx)\\
    &= \arg\max_{\vx \in \cE} \sum_{s} u_s(\vx) + \sum_{s=1}^{t-1} \widehat{u}_t(\vx)\\
\end{aligned}
\end{equation*}
\begin{equation*}
    \widehat{u}_{\tau}(\vx) := u(\vx, \widehat{\vp}_{\tau})
\end{equation*}
\begin{equation*}
\begin{aligned}
    \E[R(T)] &:= \mathbb{E}[\sum_{t=1}^T u(\vx^*, f_t) - u(\vx_t, f_t)]\\
    &= \E[\sum_{\tau=1}^Z \sum_{t \in B_\tau} u(\vx^*, f_t) - u(\vx_t, f_t)]\\
    &\leq ZK + \E[\sum_{\tau=1}^Z \sum_{t \in B_\tau} u(\vx^*, f_t) - u(\vx_{\tau}, f_t)]\\
    &= ZK + \frac{T}{Z} \cdot \sum_{\tau=1}^Z \E[u(\vx^*, \widehat{\vp}_{\tau}) - u(\vx_{\tau}, \widehat{\vp}_{\tau})]\\
    &\leq ZK + \frac{T}{Z} \left( \sum_{\tau=1}^Z \E\E_{\{\widehat{\vq}\}}[u(M(\{\widehat{\vq}\} \cup \{\widehat{\vp}_t\}_{t \leq \tau}), \widehat{\vp}_{\tau}) - u(M(\{\widehat{\vq}\} \cup \{\widehat{\vp}_t\}_{t < \tau}), \widehat{\vp}_{\tau})] \right. \\ 
    &+ \left. \E\E_{\{\widehat{\vq}\}} \left[\sum_{\widehat{\vq}_s \in \{\vq\}} 2\|\widehat{\vq}_s\|_1 \right] \right)
\end{aligned}
\end{equation*}
where the fourth line follows from Theorem 8 in~\citet{daskalakis2016learning} and the fifth line follows from the following lemma:
\begin{lemma}
    \begin{equation*}
        \E[u(\vx, \widehat{\vp}_{\tau}) - u(\vx_{\tau}, \widehat{\vp}_{\tau})] = \frac{1}{\tau} \sum_{t \in B_{\tau}} \E[u(\vx, f_t) - u(\vx_{\tau}, f_t)]
    \end{equation*}
\end{lemma}
\begin{proof}
    \begin{equation*}
    \begin{aligned}
        \E[u(\vx, \widehat{\vp}_{\tau}) - u(\vx_{\tau}, \widehat{\vp}_{\tau})] &= \E[\sum_{a_f \in \cA_f} \widehat{\vp}_{\tau}(a_f | \vx) u(\vx, a_f) - \widehat{\vp}(a_f | \vx_{\tau}) u(\vx_{\tau}, a_f)]\\
        &= \sum_{a_f \in \cA_f} \E[\widehat{\vp}_{\tau}(a_f | \vx)] u(\vx, a_f) - \E[\widehat{\vp}(a_f | \vx_{\tau})] \E[u(\vx_{\tau}, a_f)]\\
        &= \sum_{a_f \in \cA_f} \vp_{\tau}(a_f | \vx)] u(\vx, a_f) - \vp(a_f | \vx_{\tau})] \E[u(\vx_{\tau}, a_f)]\\
        &= \frac{1}{\tau} \sum_{t \in B_{\tau}} \sum_{a_f \in \cA_f} \E[\mathbbm{1}\{b_{f_t}(\vx) = a_f\} u(\vx, a_f) - \mathbbm{1}\{b_{f_t}(\vx_{\tau}) = a_f\} u(\vx_{\tau}, a_f)]\\
        &= \frac{1}{\tau} \sum_{t \in B_{\tau}} \E[u(\vx, f_t) - u(\vx_{\tau}, f_t)]
    \end{aligned}
    \end{equation*}
\end{proof}
Next steps:
\begin{itemize}
    \item Figure out which perturbation leads to stability
    \item Adopt analysis of~\citet{dani2006robbing} to nonlinear setting to get better rates (and adaptive adversaries)
\end{itemize}
